# Supplementary material for: Electron vortex beams for chirality probing at the nanoscale
Source: arXiv:2411.05579 source file (2025-01-09)
Supplement: Supplementary file 1 [file EVB_SI_v3__Copy__for_arxiv.pdf]

# Supplemental Materials: Electron Vortex Beams for Chirality Probing at the Nanoscale

Neli Lastovickova Streshkova,\* Petr Koutenský, and Martin Kozák  
*Department of Chemical Physics and Optics, Faculty of Mathematics and Physics,  
Charles University, Ke Karlovu 3, Prague CZ-12116, Czech Republic.*

(Dated: November 8, 2024)

## I. SEMICLASSICAL MODEL OF THE DICHOIC RESPONSE

We theoretically propose a technique for measuring the chirality of nanoscale systems. A chiral electron beam which is a superposition of electron vortex states with shifted OAM and momentum is used as a probe that is interacting with a chiral optical near-field. The free electron spectra after the interaction with the near-field exhibit dichroism with respect to the chirality of the near-field. In the main article we explain the dichroic response quantum mechanically through the interference of different quantum state ladders (see Fig. 2 in the article) and classically as the effect of Lorentz force.

To aid the understanding of the physics behind this dichroic response we present a detailed graphic explanation on the chirality of the ponderomotive potential, the near-field and the free electron beam itself.

In the theoretical description we follow the semi-classical framework. The interactions between the electrons and the optical fields are described in terms of perturbation theory, where the interaction leads to periodic phase modulation of the initial quasi-monochromatic wave function. The periodic phase modulation can be then decomposed into a sum Fourier components corresponding to the generated of energy side-bands in the free electron spectrum. The amplitudes and phases of the generated states are given by the interaction strength parameters  $g_{\omega}^{(1)}$  and  $g_{\omega}^{(2)}$ , defined explicitly in the main article, see Eq. (17) and Eq. (22).

In Fig. S1 we show the calculated  $g_{\omega}^{(1)}$  in the ponderomotive interaction site for several different cases. For collinear geometry (when the optical fields generating the ponderomotive potential are counter-propagating)  $g_{\omega}^{(1)}$  has axially symmetric amplitude and phase factor proportional to  $e^{\pm i\varphi}$  for OAM of the optical beam  $\hbar$  (a,b) and  $-\hbar$  (c,d). The result for noncollinear geometry and OAM  $\hbar$  is shown in (e,f), where we can see that the amplitude profile is deformed. There is also very slight change in the phase profile. For the experimental feasibility of the proposed scheme analysis we will later also discuss the effect of partially spatially correlated random noise ( $g_{\omega}^{(1)}$  with 30% random noise in the amplitude and phase is shown in (g,h)) and lateral misalignment of the optical vortex with respect to the  $z$  axis (in (i,j) we show the calculation for  $1.5 \mu\text{m}$  misalignment in the  $x$  direction).

In Fig. S2 we show the calculated  $g_{\omega}^{(2)}$  for 4 different geometries. In Fig. S2(a,b)  $g_{\omega}^{(2)}$  is calculated for left-hand circularly polarized illumination of the golden nanosphere, incident along the  $z$  axis. We note that the phase has the same sense of rotation as the phase of the ponderomotive potential (Fig. S1(b)), hence the term “co-rotating, collinear geometry”. In Fig. S2(c,d) the nanosphere is illuminated by right-hand circularly polarized plane wave propagating along the  $z$  axis. We note that the phase has now the opposite sense of rotation with respect to (Fig. S1(b)), hence the term “counter-rotating, collinear”. In Fig. S2(e,f) the nanosphere is illuminated by left-hand circularly polarized plane wave incoming from an angle with respect to the  $z$  axis, to which we refer as “co-rotating, noncollinear” geometry. In Fig. S2(g,h) the nanosphere is illuminated by linearly polarized light along the  $z$  axis, resulting in an achiral  $g_{\omega}^{(2)}$ .

Another way to understand the chirality of the near-field is by calculating the OAM spectrum of  $g_{\omega}^{(1,2)}$ . We calculate the OAM components  $G_{\omega}^{(1,2)}(l)$  as

$$G_{\omega}^{(1,2)}(l) = \frac{\int_0^{\infty} \int_0^{2\pi} R dR d\varphi g_{\omega}^{(1,2)}(R, \varphi) \exp[-il\varphi]}{\int_0^{\infty} \int_0^{2\pi} R dR d\varphi |g_{\omega}^{(1,2)}(R, \varphi)|}. \quad (\text{S1})$$

The OAM spectra of  $g_{\omega}^{(1)}$  are shown in Fig. S3. For the collinear noiseless case (Fig. S3(a,b)), the topological charge is purely  $\pm 1$ , depending on the OAM of the optical vortex. For the noncollinear case (Fig. S3(c)), there is only a

---

\* neli.streshkova@matfyz.cuni.cz

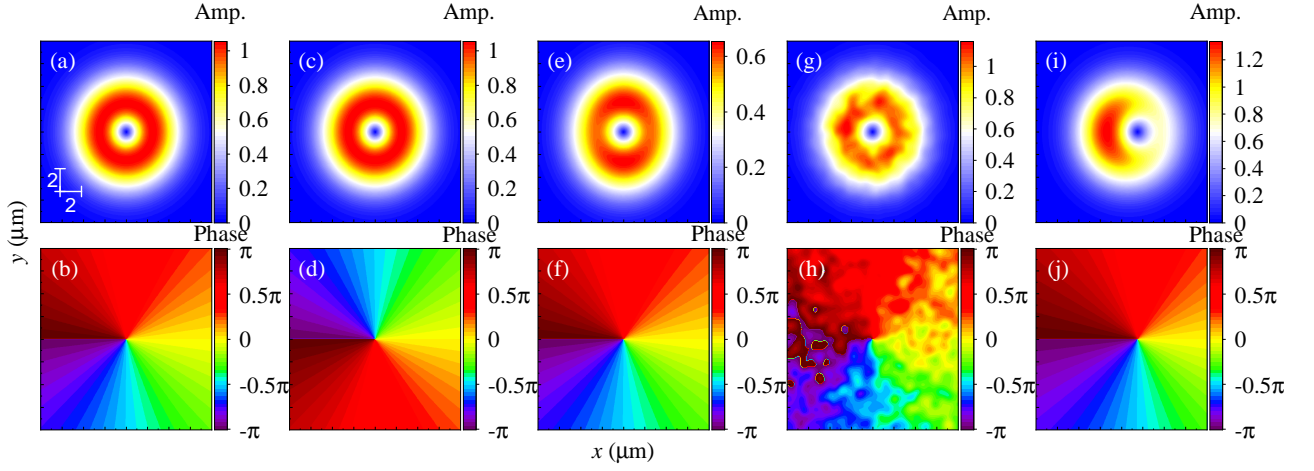

FIG. S1. Examples of the calculated  $g_{\omega}^{(1)}$  interaction parameter. We consider collinear geometry with OAM  $+\hbar$  (a,b) and OAM  $-\hbar$  (c,d) of the optical beam. In (c,f) the parameter is calculated for  $+\hbar$  OAM of the optical beam incident under angle  $\alpha = 13.4^\circ$ . In (g,h) noise is added to the amplitude and phase for collinear geometry, OAM  $+\hbar$ . In (i,j) the optical vortex axis is shifted by  $1.5 \mu\text{m}$ .

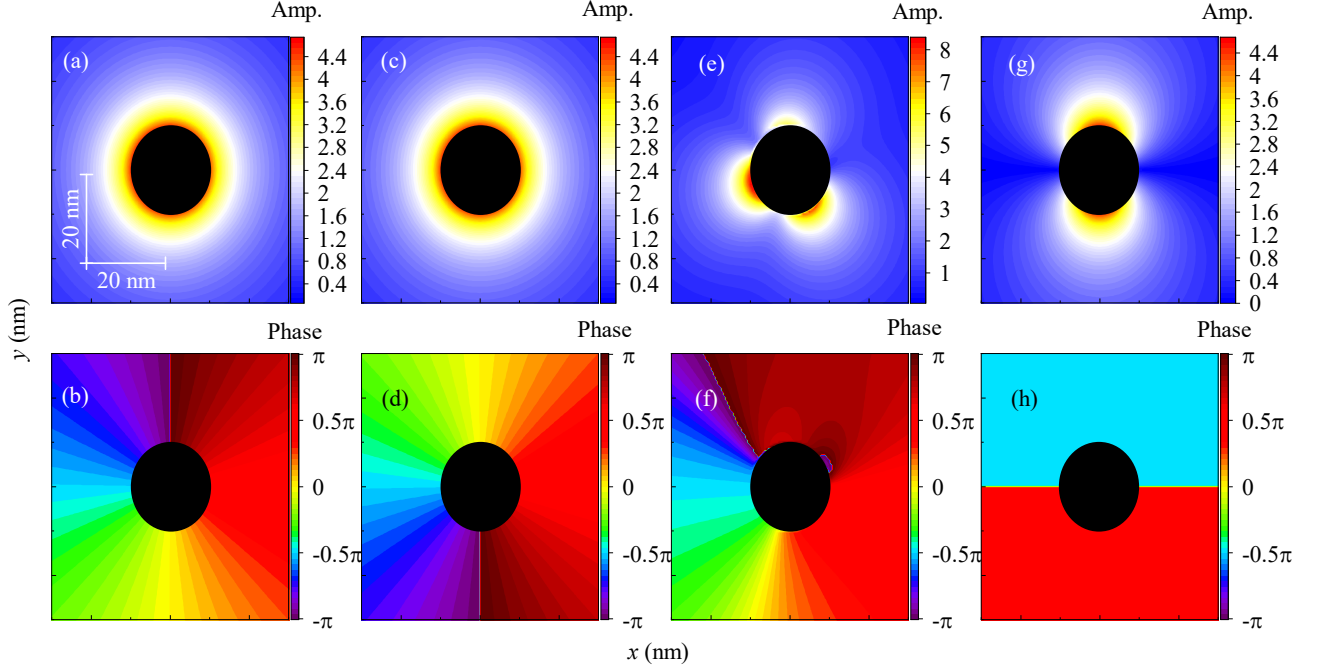

FIG. S2. Examples of the calculated  $g_{\omega}^{(2)}$  interaction parameter. We consider co-rotating, collinear excitation of the nanosphere (a,b) and counter-rotating, collinear excitation of the nanosphere (c,d). In (e,f) the parameter is calculated for co-rotating, collinear excitation of the nanosphere with the optical beam incident under angle  $\alpha = 13.4^\circ$ . In (g,h) noise is added to the amplitude and phase for collinear geometry, OAM  $+\hbar$ . In (i,j) we show an example achiral (linearly polarized) excitation. The black circles correspond to the geometric shadow of the nanosphere.

slight decrease (less than 0.1 %) in the amplitude of the  $l = 1$  state. We calculated that 30% noise in the amplitude and the phase (Fig. S3(d)) yields decrease of approximately 7%. The  $1.5 \mu\text{m}$  misalignment (Fig. S3(e)) leads to more noticeable decrease of the vortex purity, with  $l = 0$  and  $l = 2$  states additionally present.

The OAM spectra of  $g_{\omega}^{(2)}$  for the golden nanosphere and nanostructures studied in the article are shown in Fig. S4. For collinear geometry of the nanosphere excitation the co-rotating and counter-rotating near-fields have sharp OAMs of 1 and -1 respectively (Fig. S4(a,b)). For the non-collinear case (Fig. S4(c)) besides the  $l = 1$  there are contributions from higher OAM values. For the achiral case with linear excitation of the sphere there is equal weight

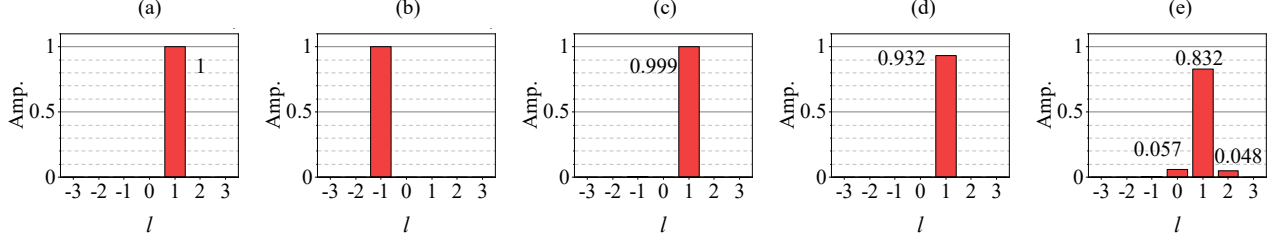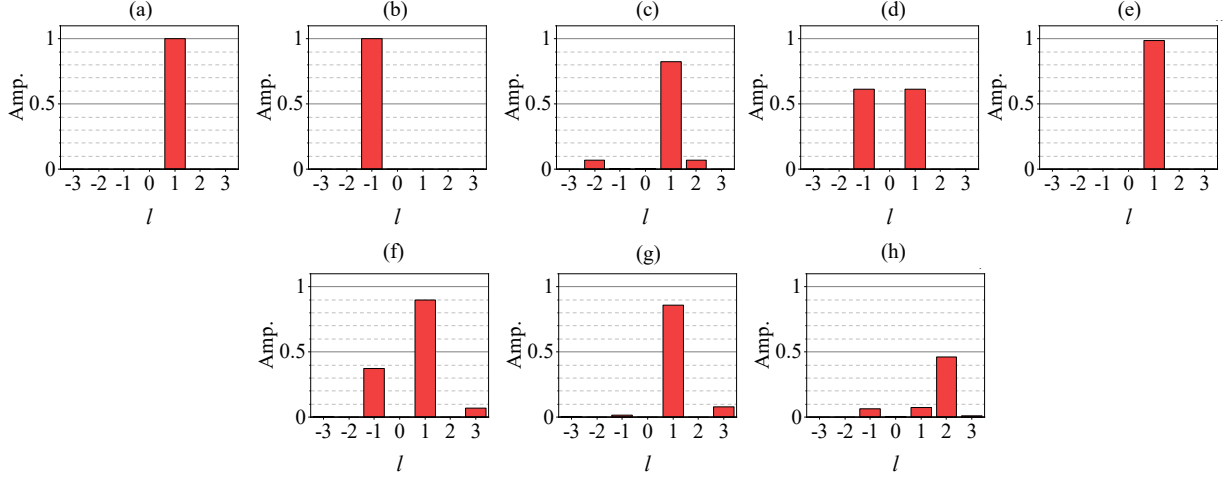

FIG. S4. OAM spectra of the  $g_{\omega}^{(2)}$  interaction parameter: (a) collinear co-rotating excitation of the nanosphere, (b) collinear counter-rotating excitation of the nanosphere, (c) co-rotating excitation of the nanosphere with optical beam incident under angle  $\alpha = 13.4^\circ$ , (d) collinear, linearly polarized excitation of the nanosphere, (e) collinear co-rotating excitation of the nanosphere placed on a  $\text{Si}_3\text{N}_4$  membrane, (f) collinear, linearly polarized excitation of the two nanorod nanostructure, (g) collinear, linearly polarized excitation of the nanorod helix nanostructure, (h) collinear, linearly polarized excitation of the nanosphere helix nanostructure. The counterparts of the nanostructures with opposite chiralities have OAM spectra mirrored around the  $l = 0$  point.

of OAM 1 and -1 (Fig. S4(d)). For completeness, we also show the calculated the OAM spectrum for co-rotating collinear excitation of the nanosphere placed on a 200 nm  $\text{Si}_3\text{N}_4$  membrane (the near-field was simulated numerically using the FDTD method) (Fig. S4(e)), where the normalized amplitude of the  $l = 1$  state has decreased to  $\approx 0.99$  from the amplitude of 1 for the vacuum case.

The nanostructures presented in the article (Fig. 8) produce chiral near-fields after being illuminated with linearly polarized light. The OAM spectrum of the two nanorod structure (Fig. S4(f)) has dominant contribution from the  $l = 1$  state, however  $l = -1$  and  $l = 3$  contributions are present, which decreases the OAM purity. The OAM spectrum of the nanorod helix (Fig. S4(g)) has better OAM purity for  $l = 1$ . The OAM spectrum of the nanosphere helix (Fig. S4(h)) has equal contributions from  $l = -1$  and  $l = +1$ , which suggests that it would behave like achiral structure when probed with electron beam generated with OAM  $\pm\hbar$  optical vortex. For this structure the dominant contribution is from  $l = 2$ , which is sensitive to electron probe generated with OAM  $\pm 2\hbar$  optical vortex.

The ideal case when the free electron dichroism is most pronounced corresponds to a situation in which the topological charges are pure for both  $g_{\omega}^{(1)}$  and  $g_{\omega}^{(2)}$ . The mixing of other topological states leads to the decrease of the dichroism.

Now let us see how the chirality of the fields translates into the electron beam. We suppose that the initial beam has Gaussian profile shown in Fig. S5(a). According to Eq. (16) in the article the ponderomotive interaction leads to the generation of energy side-bands, with different momenta and orbital angular momenta. For OAM of the optical vortex  $+\hbar$  the energy states with higher energies and momenta have positive OAMs. For OAM of the optical vortex

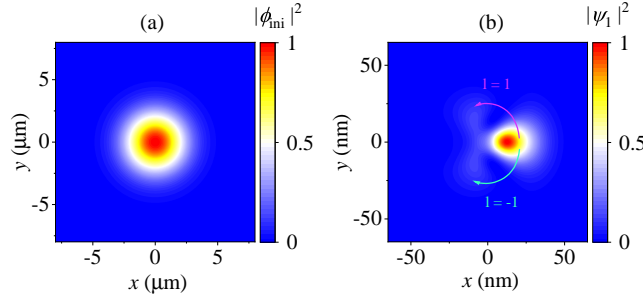

FIG. S5. Probability density of the electron beam (a) before interaction with the ponderomotive potential and (b) after interaction with the ponderomotive potential and focusing onto the second interaction plane. The probability density is captured for fixed time  $t$  and with evolving time rotates around the origin counter-clockwise ( $l=1$ ) or clockwise ( $l=-1$ ).

$-1\hbar$  the energy states with higher energies and momenta have negative OAMs. The individual vortex states propagate dispersively, leading to bunching in the temporal profile with period  $2\pi/\omega$ . This bunching is phase dependent, so for constant position  $z$  we can see the electron probability density rotate with period  $2\pi/\omega$  in the  $xy$  plane. The shape of the focused superposition of states in position  $z = d$  is shown in Fig. S5(b). For OAM of the ponderomotive interaction parameter  $+\hbar$  the probability density rotates counter-clockwise (seen against the direction of propagation) and clockwise for  $-\hbar$ . The electron beam itself is chiral.

Further we inspect the effect of the interaction with the near-field. For simplicity, we discuss the collinear geometry without any misalignments or noise. In Fig. S6 we show the real space decomposition of the wave function into the three central bands  $k = -1, 0, 1$ . The probability densities of the individual states are scaled by a common factor for each row. Prior to interacting with the near-field all the three components have radially symmetric probability densities as shown in Fig. S6(a,b,c).

When interacting with a near-field, the wave function is described by Eq. (21) in the article. The profile of the newly generated  $k$  states (corresponding to shift  $k\hbar\omega$  in energy) depends on the phase difference between the interaction parameters in the first and second site. For the near-field that has the same OAM as the ponderomotive interaction field (Fig. S6(d,e,f)) this phase difference is constant over the transverse plane, hence the transverse profile of the new energy is also radially symmetric. However, for this particular phase difference ( $\pi/2$ ) most of the electrons are transferred to the  $k = -1$  state. On the contrary, if the near-field has an opposite OAM with respect to the ponderomotive field (Fig. S6(g,h,i)), the relative phase between the two interaction parameters changes within the transverse plane and generates an equal amount of  $k = -1$  and  $k = +1$  electrons when integrated over the electron beam profile. The position of the "lobes" is dependent on the mutual phase between the two interactions.

This effect can be easily explained in a simplified analytical model. Let us suppose we have two space-separated interactions with mutual distance  $d$  with the same modulation frequency  $\tilde{\omega}$  and interaction parameters  $f^{(1)}$  and  $f^{(2)}$ . For simplicity consider that the two interactions have comparable sizes and we can omit the beam focusing. Further we suppose that both the interactions are weak, so  $J_k(f^{(1,2)}) \approx 0$  for  $k \geq 2$ . The wave function  $\xi$  immediately after the second interaction is

$$\xi(R, \varphi, z = d, t) = \sum_{k=-1}^1 \sum_{k'=-1}^1 \left[ J_k(2|f^{(1)}|) e^{ik \arg f^{(1)}} e^{-i(k\tilde{\omega}t - k\frac{\tilde{\omega}}{v}d + 2\pi k^2 \frac{d}{z_T})} J_{k'}(2|f^{(1)}|) e^{ik' \arg f^{(1)}} e^{-i(k'\tilde{\omega}t)} \right]. \quad (\text{S2})$$

For example, we can choose only the terms contributing to the  $k = 1$  energy side band (the one that has time oscillation factor  $e^{-i\tilde{\omega}t}$ ). Then the probability density for this particular momentum state  $\xi_1$  is

$$|\xi_1|^2 = |J_0(2|f^{(2)}|)J_1(2|f^{(1)}|)|^2 + |J_0(2|f^{(1)}|)J_1(2|f^{(2)}|)|^2 + 2 \left[ J_0(2|f^{(2)}|)J_1(2|f^{(1)}|)J_1(2|f^{(2)}|)J_0(2|f^{(1)}|) \right] \cos \left[ \arg f^{(1)} - \arg f^{(2)} + \tilde{\omega}d/v - 2\pi d/z_T \right]. \quad (\text{S3})$$

For the  $k = -1$  momentum state probability density we can write

$$|\xi_{-1}|^2 = |J_0(2|f^{(2)}|)J_{-1}(2|f^{(1)}|)|^2 + |J_0(2|f^{(1)}|)J_{-1}(2|f^{(2)}|)|^2 + 2 \left[ J_0(2|f^{(2)}|)J_{-1}(2|f^{(1)}|)J_{-1}(2|f^{(2)}|)J_0(2|f^{(1)}|) \right] \cos \left[ -\arg f^{(1)} + \arg f^{(2)} - \tilde{\omega}d/v - 2\pi d/z_T \right]. \quad (\text{S4})$$

Setting  $\arg f^{(1)} = \varphi + \Delta\varphi$  and  $\arg f^{(2)} = \varphi$  we model the collinear co-rotating case, where the phases of the two

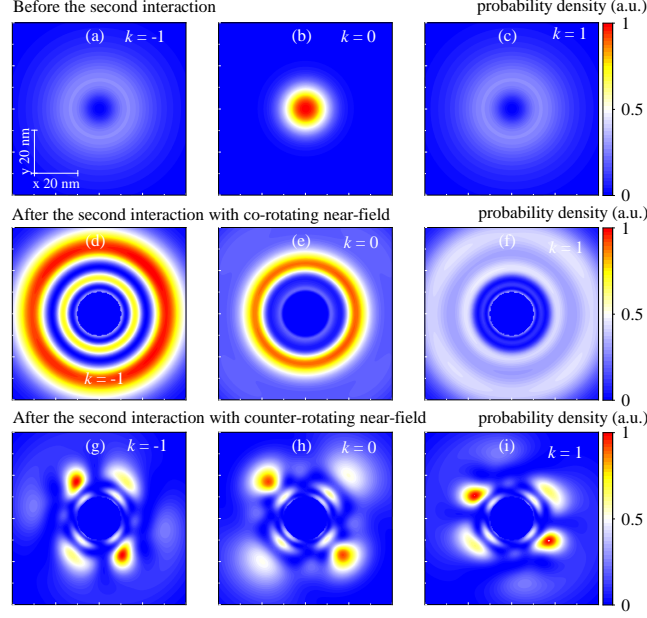

FIG. S6. Energy filtered images of the energy/momentum states of the electron wave function (a,b,c) focused in the second interaction site, (d,e,f) after interaction with a co-rotating near-field, (g,h,i) after interaction with counter-rotating near-field.

interactions differ by a constant factor. This explains the radial symmetry.

$$|\xi_1|^2 = |J_0(2|f^{(2)}|)J_1(2|f^{(1)}|)|^2 + |J_0(2|f^{(1)}|)J_1(2|f^{(2)}|)|^2 + 2 \left[ J_0(2|f^{(2)}|)J_1(2|f^{(1)}|)J_1(2|f^{(2)}|)J_0(2|f^{(1)}|) \right] \cos \left[ \Delta\varphi + \tilde{\omega}d/v - 2\pi d/z_T \right]. \quad (\text{S5})$$

$$|\xi_{-1}|^2 = |J_0(2|f^{(2)}|)J_{-1}(2|f^{(1)}|)|^2 + |J_0(2|f^{(1)}|)J_{-1}(2|f^{(2)}|)|^2 + 2 \left[ J_0(2|f^{(2)}|)J_{-1}(2|f^{(1)}|)J_{-1}(2|f^{(2)}|)J_0(2|f^{(1)}|) \right] \cos \left[ \Delta\varphi + \tilde{\omega}d/v + 2\pi d/z_T \right]. \quad (\text{S6})$$

Here we also see the importance of the higher order term in the momentum expansion  $i2\pi k^2 z/z_T$ . The probability density is different for  $\xi_1$  and  $\xi_2$ , because of the different argument of the cosine.

Setting  $\arg f^{(1)} = \varphi + \Delta\varphi$  and  $\arg f^{(2)} = -\varphi$  we model the collinear counter-rotating case, and the phase difference of the two interactions is a function of  $\varphi$ . For the  $k = 1$  state the cosine term takes the form  $\cos \left[ 2\varphi + \Delta\varphi + \tilde{\omega}d/v - 2\pi d/z_T \right]$  and for the  $k = -1$  state it can be written as  $\cos \left[ 2\varphi + \Delta\varphi + \tilde{\omega}d/v + 2\pi d/z_T \right]$ . Including the interaction of higher states naturally leads to a more complicated structure of the transverse profiles of the energy states.

The last step to obtain the final free electron spectra is to take the average over the entire beam profile by plugging into Eq. (24) in the article. Considering the transverse beamlet profiles it is obvious why the electron spectra after two co-rotating interactions are in general asymmetric and the spectra after two counter-rotating interactions are symmetric.

## II. EFFECTS OF AMPLITUDE AND PHASE DISTORTIONS

The vortex state is robust thanks to its topology. However, in a realistic setup there are many factors that can influence and potentially decrease the free electron spectra dichroism. The electron beam needs to have sufficient coherence properties, it needs to be spatially overlapped with two optical beams for the generation of the vortex state superposition, then it needs to be focused onto a nano-scale structure and again has to be overlapped with the scattered near-field of the nanostructure. It is necessary that the optical beams are synchronized, have stable and controllable phase delays and are long enough so the electron beam is modulated as homogeneously as possible within the duration of both of the interactions.

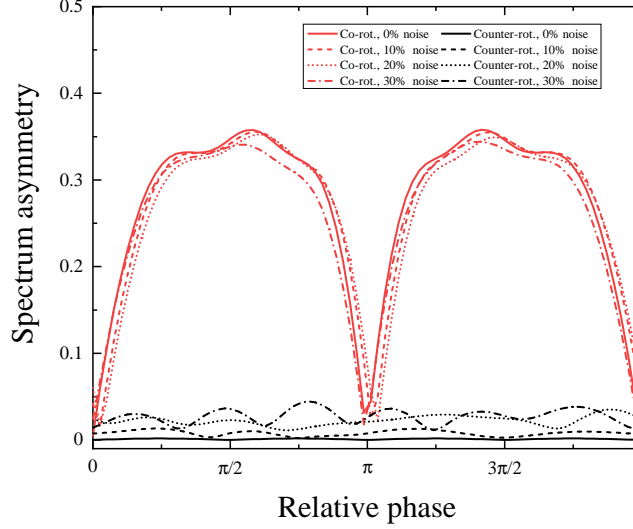

FIG. S7. Asymmetry parameters calculated from the free-electron spectra for 0%, 10%, 20% and 30% added random noise to the interaction parameter  $g_{\omega}^{(1)}$ .

In the optimal case, where everything is aligned perfectly and the geometry is collinear, thanks to the high symmetry the dichroism is most pronounced. In the main article we address two special cases deviating from the perfect situation. First we address the effect of having the optical beams incident under nonzero angles with respect to the  $z$  axis. The optical beam exciting the nanosphere is incident under the same angle as the optical vortex. Then we study the effect of axial misalignment of the studied nanosphere and the decrease of the dichroic response.

So far we supposed the electron probe consists of perfect vortex sub-states (although the wavefront is tilted for the noncollinear case). However under realistic conditions, the vortex quality is not perfect. We simulate the disrupted OAM state superposition through introducing errors in the  $g_{\omega}^{(1)}(R, \varphi)$  profile, that are then imprinted also on the electron state superposition (see Eq. (16) and also affect the focusing (Eq. (19)).

One option is to introduce random noise. Typically random phase and amplitude distortions can be expected in  $g_{\omega}^{(1)}$ , that are result of the partial coherence of the optical beams generating the ponderomotive grating. We inspect the interaction for noise levels of 10%, 20% and 30% of both the amplitude and the phase. In Fig. S1(g,h) we show an example of the interaction parameter with 30% noise and in Fig. S3(d) we show the calculated OAM spectrum.

The second option is to consider slight misalignment of the optical vortex with respect to the  $z$  axis. We calculate the effect of axial misalignment of 10%, 20% and 30% of the beam radius  $w_{\text{ini}}$ . The transverse profile of the  $g_{\omega}^{(1)}$  parameter with misalignment  $30\%w_{\text{ini}}$  in the  $x$  direction is shown in Fig S1(i,j) and the calculated OAM spectrum is shown in Fig. S3(e).

The effect of these two kinds of distortions is clearly seen in the spectrum asymmetry parameter (Fig. S7 and Fig. S5). In both cases the free electron spectra asymmetry dichroism is present. Based on the simulations we conclude that the method appears to be robust with respect to random noise, as the asymmetry changes only slightly. With the beam axial misalignment the asymmetry dichroism decreases similarly as in the case when the electron beam is perfect and the nanosphere is misaligned with respect to the  $z$  axis.

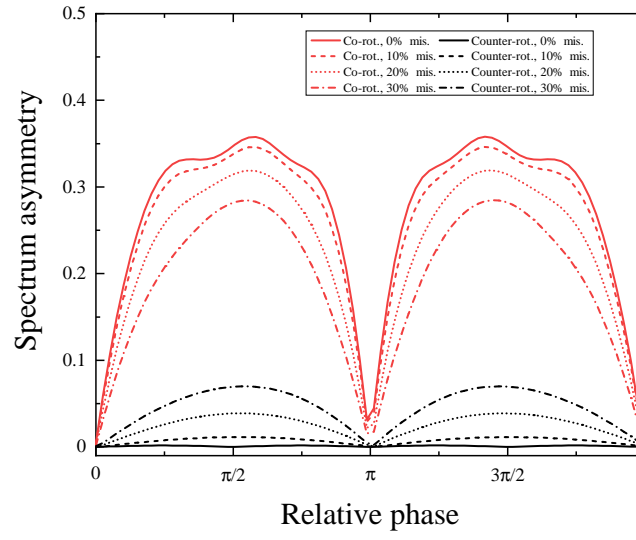

FIG. S8. Asymmetry parameters calculated from the free-electron spectra for 0%, 10%, 20% and 30% of  $w_{\text{ini}}$  misalignment in the  $x$  direction of the optical vortex generating the ponderomotive grating.
